# Supplementary material for: Enhancing two-photon spontaneous emission in rare earths using graphene and graphene nanoribbons
Source: arXiv:2212.12066 source file (2022-12-22)
Supplement: Supplementary file 1 [file 2PSE_Paper_-_Supplemental.pdf]

Supplemental Material for
"Enhancing two-photon spontaneous emission in rare earths using graphene and graphene nanoribbons"

Colin Whisler, Gregory Holdman, D. D. Yavuz, and Victor W. Brar
*University of Wisconsin-Madison, Department of Physics,*
*1150 University Ave., Madison, Wisconsin 53706, USA*

**Contents**

I. Derivation of dipole transition matrix elements
II. Variation of Purcell enhancement with dipole position
III. Variation of Purcell enhancement with dipole orientation
IV. Variation of Purcell enhancement with graphene nanoribbon width
V. Emission of mixed radiative/nonradiative modes
VI. Variation of total decay rate with graphene nanoribbon width
References

## I. Derivation of dipole transition matrix elements

As shown in Eqs. 2 and 3 of the main paper, the enhancement of the differential 2PSE rate of an emitter at frequency ω and position $r$, with single-transition frequency $\omega_0$, is given by

$$\frac{\gamma(\omega,\mathbf{r})}{\gamma_0(\omega)} = \frac{\sum_{i,j}|D_{ij}(\omega,\omega_0-\omega)|^2 P_i(\omega,\mathbf{r})P_j(\omega_0-\omega,\mathbf{r})}{\sum_{i',j'}|D_{i'j'}(\omega,\omega_0-\omega)|^2} \tag{S1}$$

where $P_i(\omega, r)$ represents the Purcell enhancement of an emitter oriented along the $i$-axis with frequency ω and position $r$, and

$$D(\omega_1,\omega_2) = \sum_n \left(\frac{\mathbf{d}_{ne}\mathbf{d}_{gn}}{\omega_n-\omega_e+\omega_1} + \frac{\mathbf{d}_{gn}\mathbf{d}_{ne}}{\omega_n-\omega_e+\omega_2}\right). \tag{S2}$$

Here, $\hbar\omega_n$ and $\hbar\omega_e$ represent the energy levels of the intermediate state $n$ and the excited state $e$, respectively, and the three components of the vector $\mathbf{d}_{ne}$ are the electric dipole matrix elements $\langle n|\mathbf{x}|e\rangle$, $\langle n|\mathbf{y}|e\rangle$, and $\langle n|\mathbf{z}|e\rangle$ connecting the excited state to the intermediate state. $\mathbf{d}_{gn}$ is similar, connecting $n$ to the ground state $g$.

The form of the matrix $D(\omega_1, \omega_2)$ will depend on the emitter's atomic structure. For a hydrogenic ion with excited and ground states in the $s$ configuration, the only intermediate states with nonzero matrix elements are those in the $p$ configurations. An intermediate $p_x$ state will only allow nonzero values for the x-components of $\mathbf{d}_{ne}$ and $\mathbf{d}_{gn}$, and likewise for the $p_y$ and $p_z$ states, causing $D(\omega_1, \omega_2)$ to be diagonal in these systems. Meanwhile, the states of rare earth ions such as $Er^{3+}$ have multiple electrons in $4f$ orbitals, along with $5d$ and $6s$ for excited states. It can therefore be possible for a

single intermediate state to be connected via two transitions with different polarizations. $D(\omega_1, \omega_2)$ will no longer be diagonal for these systems; however, symmetry does enforce some constraints on this matrix. Because $D(\omega_1, \omega_2)$ is a property only of the emitter itself, which does not have a fixed orientation in space, there should be no inherent differences between x-, y-, and z-components, with the only potential variations coming between on-diagonal elements and off-diagonal elements.

The atomic structure codes used in our analysis [1] return the oscillator strength of each transition, weighted by the number of J states. This value $gf$ is then used to find the radial matrix elements according to the relation

$$gf = \frac{8\pi^2 mca_0}{3h\lambda} \left|\langle\gamma J||r||\gamma' J'\rangle\right|^2 . \qquad \text{(S3)}$$

Here $m$ is the mass of an electron, $c$ is the speed of light, $a_0$ is the Bohr radius, $h$ is Planck's constant, $\lambda$ is the wavelength of the transition between the intermediate state and the ground (or excited) state, and $\langle\gamma J||r||\gamma' J'\rangle$ is the reduced radial matrix element. To convert these values into the x-, y-, and z-components of $\mathbf{d}_{ne}$ and $\mathbf{d}_{gn}$, we first find the irreducible tensor components using the Wigner-Eckart Theorem [2, 3]:

$$\langle\gamma JM|r_q|\gamma' J'M'\rangle = (-1)^{J-M} \begin{pmatrix} J & 1 & J' \\ -M & q & M' \end{pmatrix} \langle\gamma J||r||\gamma' J'\rangle, \qquad \text{(S4)}$$

where q=(-1, 0, 1) and the allowed M-values range from -J to +J. We find the values of these irreducible tensor components of the position operator for each transition between the excited state ${}^4I_{13/2}$ and each intermediate state in the $4f^{10}5d$ and $4f^{10}6s$ configurations, as well as between each of these intermediate states and the ground state ${}^4I_{15/2}$. Because an electric dipole transition changes J by either 0 or $\pm 1$, the only intermediate states capable of connecting to both the ground and excited states are those with either J=13/2 or J=15/2.

We now find the x-, y-, and z-components for each transition according to

$$x = \frac{1}{\sqrt{2}}(r_{-1} - r_1), \qquad \text{(S5)}$$

$$y = \frac{i}{\sqrt{2}}(r_{-1} + r_1), \qquad \text{(S6)}$$

$$z = r_0. \qquad \text{(S7)}$$

This means that the x and y matrix elements correspond to transitions where M changes by $\pm 1$, while z matrix elements correspond to transitions where M does not change. These directional matrix elements for each transition are inserted into Eq. S2 and summed over all possible intermediate states, which vary not only in their energy level but also in the identification of their M value.

To simplify our calculation of $D(\omega_1, \omega_2)$, we eliminate the dependence on the frequency by neglecting to include the contributions of $\omega_1$ and $\omega_2$ in the denominator of Eq. S2. This introduces only very minor errors to the emission enhancement, since the transition frequency $\omega_n - \omega_e$ is much larger than the emission frequency, which may range from 0 to $\omega_0$. The resulting matrix $\frac{|D_{ij}(\omega,\omega_0-\omega)|^2}{\sum_{i',j'}|D_{i'j'}(\omega,\omega_0-\omega)|^2}$ represents the relative weighting of the product of Purcell factors in the $i$ and $j$ directions; that is,

$$\frac{\gamma(\omega,\mathbf{r})}{\gamma_0(\omega)} \approx \sum_{i,j} A_{ij} P_i(\omega,\mathbf{r}) P_j(\omega_0-\omega,\mathbf{r}) \tag{S8}$$

with $A_{i,j} = \frac{|D_{ij}(\omega,\omega_0-\omega)|^2}{\sum_{i',j'}|D_{i'j'}(\omega,\omega_0-\omega)|^2}$. This matrix will have different values depending on the M values for the initial and final electron states. It takes the following values:

$$(M_f = M_i \pm 2):\begin{pmatrix} A_{xx} & A_{xy} & A_{xz} \\ A_{yx} & A_{yy} & A_{yz} \\ A_{zx} & A_{zy} & A_{zz} \end{pmatrix} = \begin{pmatrix} 1/4 & 1/4 & 0 \\ 1/4 & 1/4 & 0 \\ 0 & 0 & 0 \end{pmatrix} \tag{S9}$$

$$(M_f = M_i \pm 1):\begin{pmatrix} A_{xx} & A_{xy} & A_{xz} \\ A_{yx} & A_{yy} & A_{yz} \\ A_{zx} & A_{zy} & A_{zz} \end{pmatrix} = \begin{pmatrix} 0 & 0 & 1/4 \\ 0 & 0 & 1/4 \\ 1/4 & 1/4 & 0 \end{pmatrix} \tag{S10}$$

$$(M_f = M_i):\begin{pmatrix} A_{xx} & A_{xy} & A_{xz} \\ A_{yx} & A_{yy} & A_{yz} \\ A_{zx} & A_{zy} & A_{zz} \end{pmatrix} = \begin{pmatrix} 1/6 & 0 & 0 \\ 0 & 1/6 & 0 \\ 0 & 0 & 2/3 \end{pmatrix}. \tag{S11}$$

Finally, these terms are averaged across all allowed combinations of initial and final M values for the $Er^{3+}$ initial (J=13/2) and final (J=15/2) states, resulting in

$$\begin{pmatrix} A_{xx} & A_{xy} & A_{xz} \\ A_{yx} & A_{yy} & A_{yz} \\ A_{zx} & A_{zy} & A_{zz} \end{pmatrix} = \begin{pmatrix} 2/15 & 1/10 & 1/10 \\ 1/10 & 2/15 & 1/10 \\ 1/10 & 1/10 & 2/15 \end{pmatrix}. \tag{S12}$$

## II. Variation of Purcell enhancement with dipole position

Our main analysis focuses only on emitters located at a distance of 5 nm beneath the center of the graphene nanoribbons, where the Purcell enhancement is maximized. In an experimental setting, many emitters would instead be distributed throughout all lateral positions relative to the ribbons.

Fig. S1(a, b, c, d) shows the variation in Purcell enhancement of a dipole located 10 nm beneath an array of 20 nm graphene nanoribbons as a function of photon emission energy. The dipole is positioned beneath the center of the gap between two ribbons (pink, dotted), the edge of a ribbon (blue, dashed), and the center of a ribbon (orange, solid) for four different Fermi energies. Although the emitters located beneath the ribbon edge show additional resonances not found when positioned elsewhere, the overall enhancement is much stronger beneath the ribbon's center.

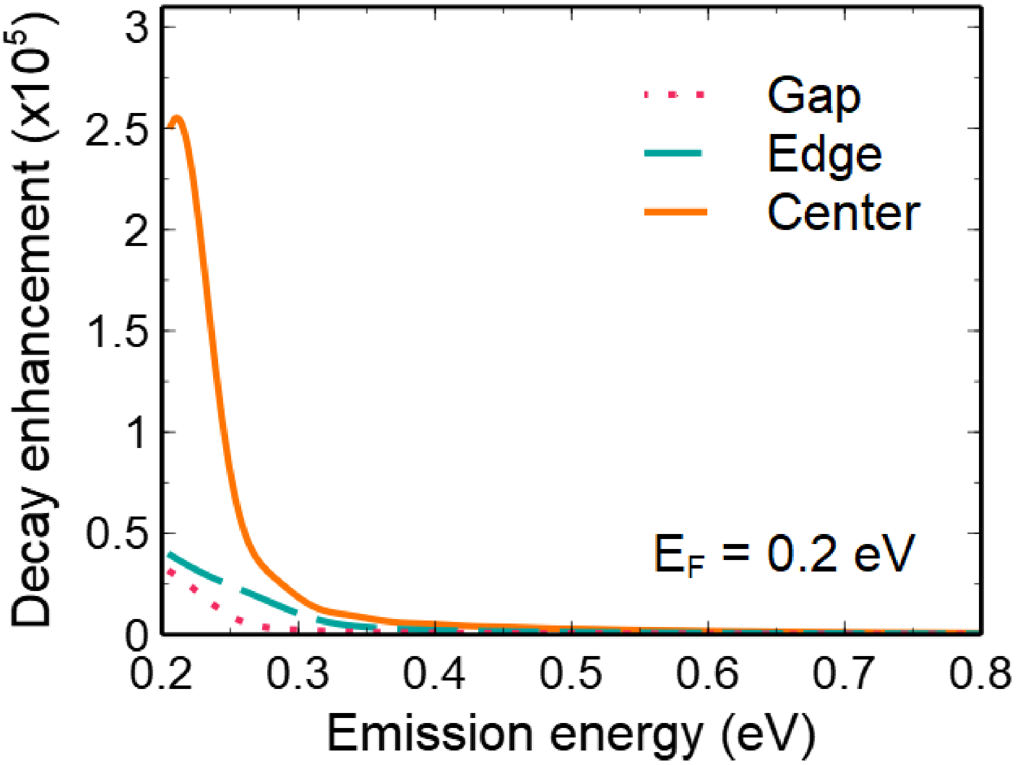

Fig. S1(a): Purcell enhancement of a dipole 10 nm beneath graphene nanoribbons at Fermi energy 0.2 eV.

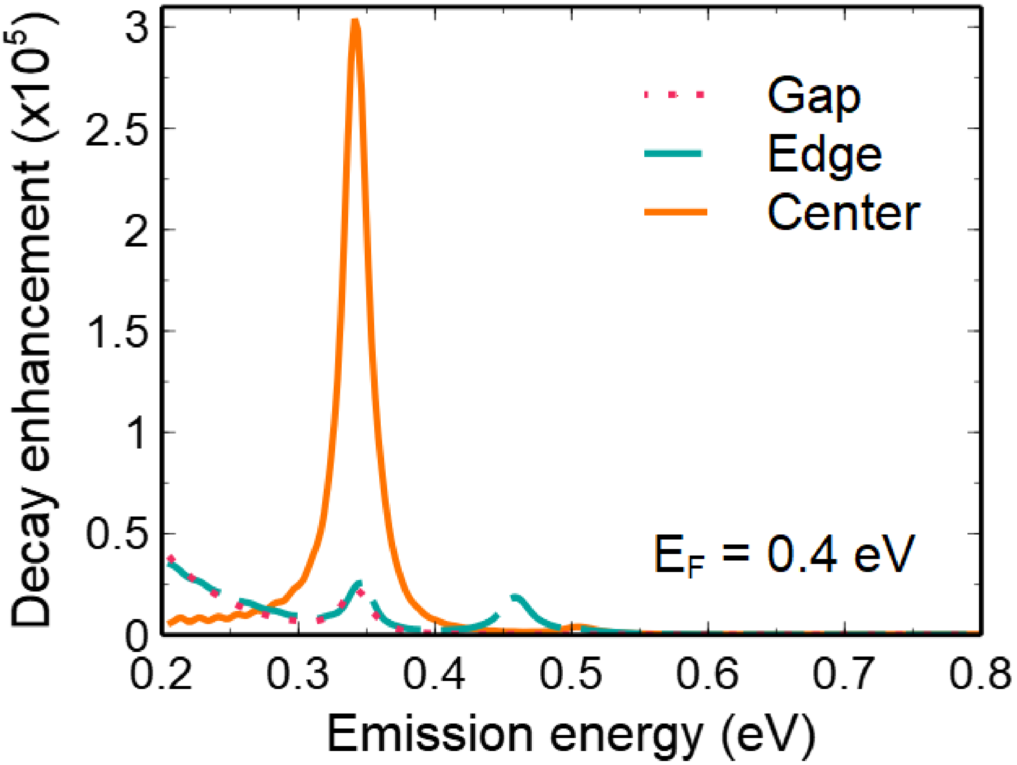

Fig. S1(b): Purcell enhancement of a dipole 10 nm beneath graphene nanoribbons at Fermi energy 0.4 eV.

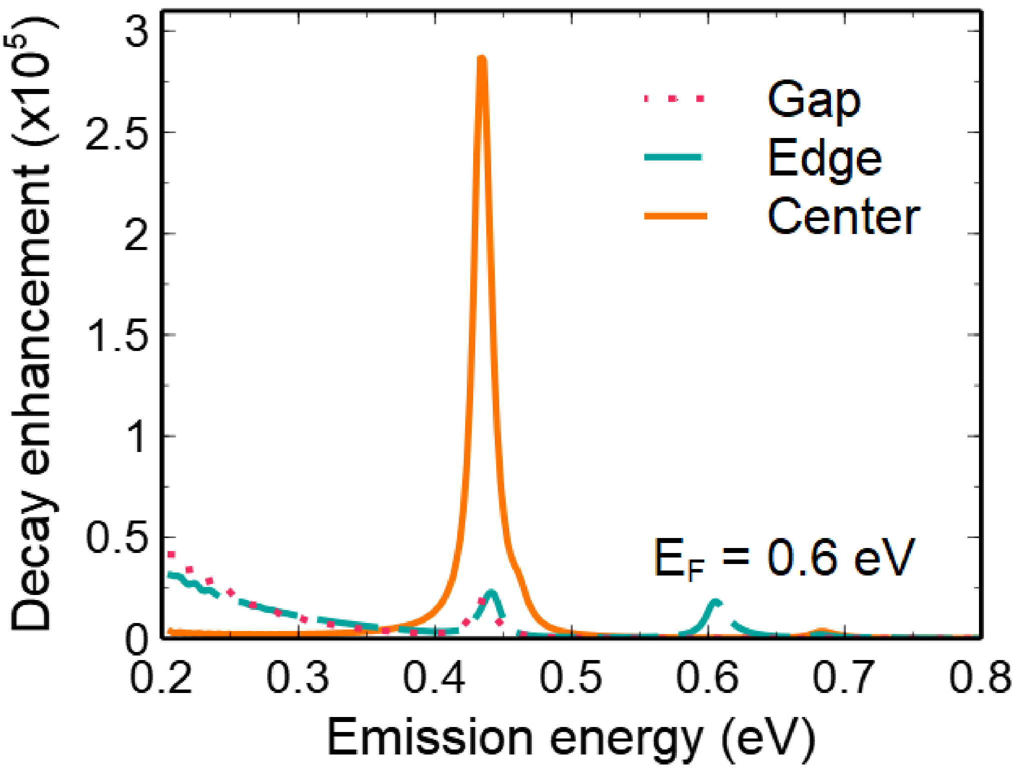


Fig. S1(c): Purcell enhancement of a dipole 10 nm beneath graphene nanoribbons at Fermi energy 0.6 eV.

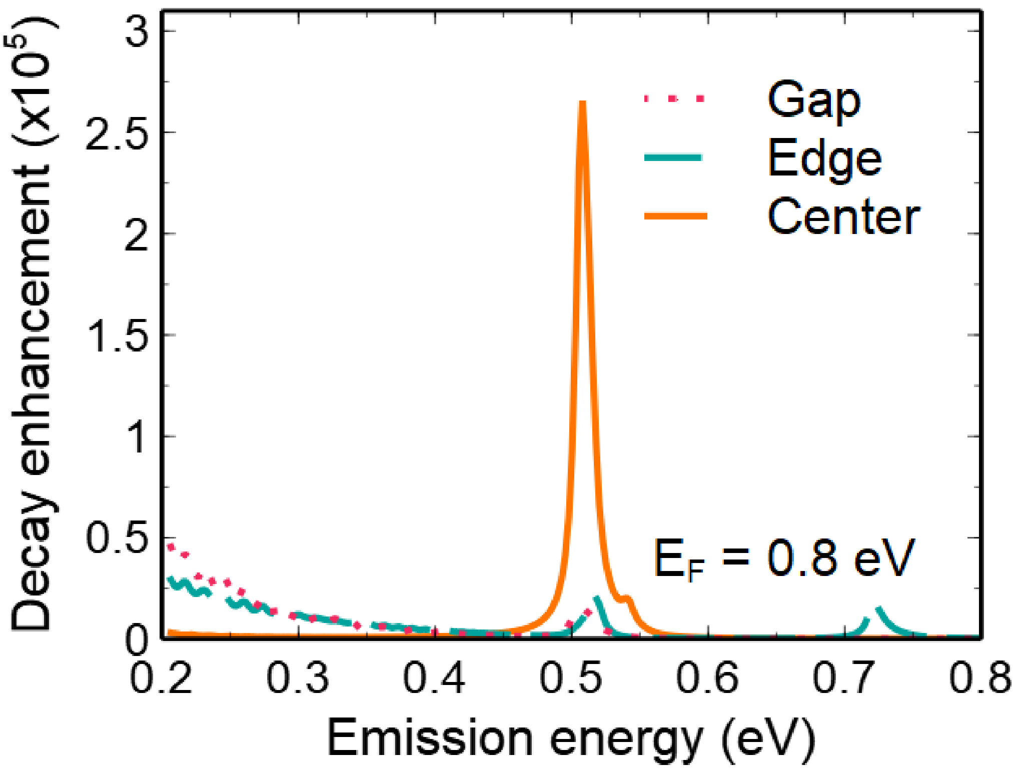


Fig. S1(d): Purcell enhancement of a dipole 10 nm beneath graphene nanoribbons at Fermi energy 0.8 eV.

## III. Variation of Purcell enhancement with dipole orientation

Fig. 2 of the main paper shows the Purcell enhancement and 2PSE enhancement of an $Er^{3+}$ emitter 5 nm beneath an array of 20 nm graphene ribbons, polarized in the x-direction. These results illustrate how Fermi energies with dual resonances in the emission frequencies experience increased enhancement of 2PSE; however, the full observed value of 2PSE enhancement (Fig. 4a) includes contributions from all dipole orientations. We thus present in Fig. S2-S4 similar results for Purcell enhancement, 2PSE enhancement, and differential 2PSE enhancement for all three polarizations of the dipole beneath 20 nm graphene ribbons and compared to a continuous graphene sheet.

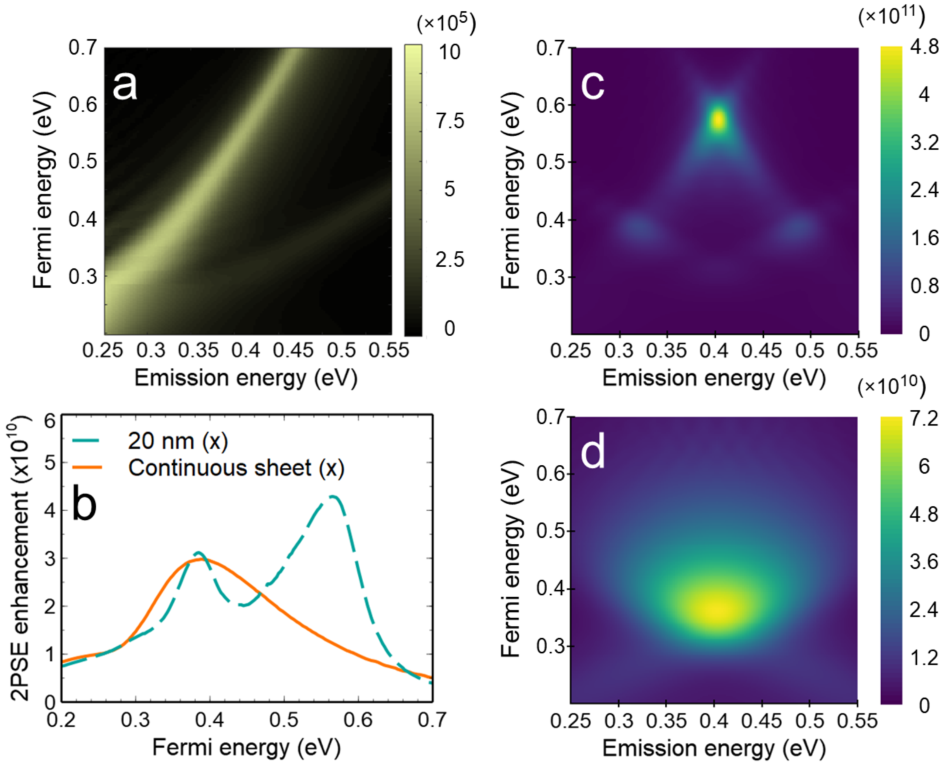


Fig. S2: Results for an emitter in the x-direction (along the ribbon's short axis or parallel to the sheet). (a) Purcell enhancement for the emitter 5 nm beneath 20 nm graphene ribbons. (b) Integrated 2PSE enhancement $\Gamma/\Gamma_0$ for the emitter near 20 nm wide graphene ribbons and near a continuous graphene sheet. (c, d) Differential 2PSE enhancement $\gamma/\gamma_{0,\max}$ for the emitter near graphene ribbons (c) or a graphene sheet (d). The results in (c) and (d) are normalized by the maximum value of free-space differential 2PSE.

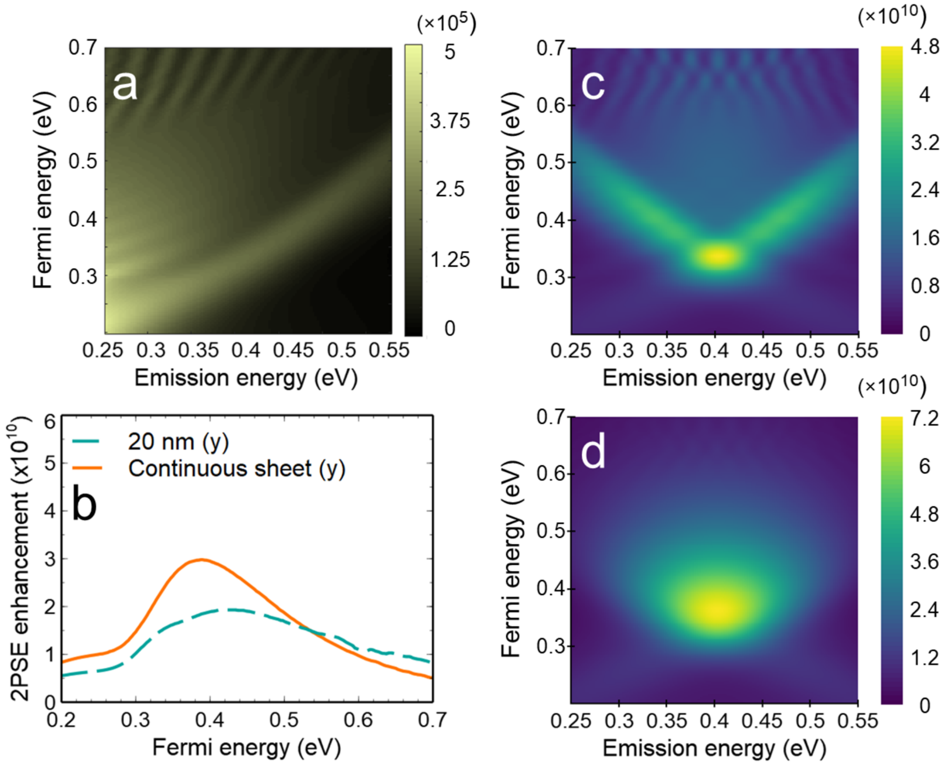


Fig. S3: Results for an emitter in the y-direction (along the ribbon's long axis or parallel to the sheet). (a) Purcell enhancement for the emitter 5 nm beneath 20 nm graphene ribbons. (b) Integrated 2PSE enhancement $\Gamma/\Gamma_0$ for the emitter near 20 nm wide graphene ribbons and near a continuous graphene sheet. (c, d) Differential 2PSE enhancement $\gamma/\gamma_{0,\max}$ for the emitter near graphene ribbons (c) or a graphene sheet (d). The results in (c) and (d) are normalized by the maximum value of free-space differential 2PSE.

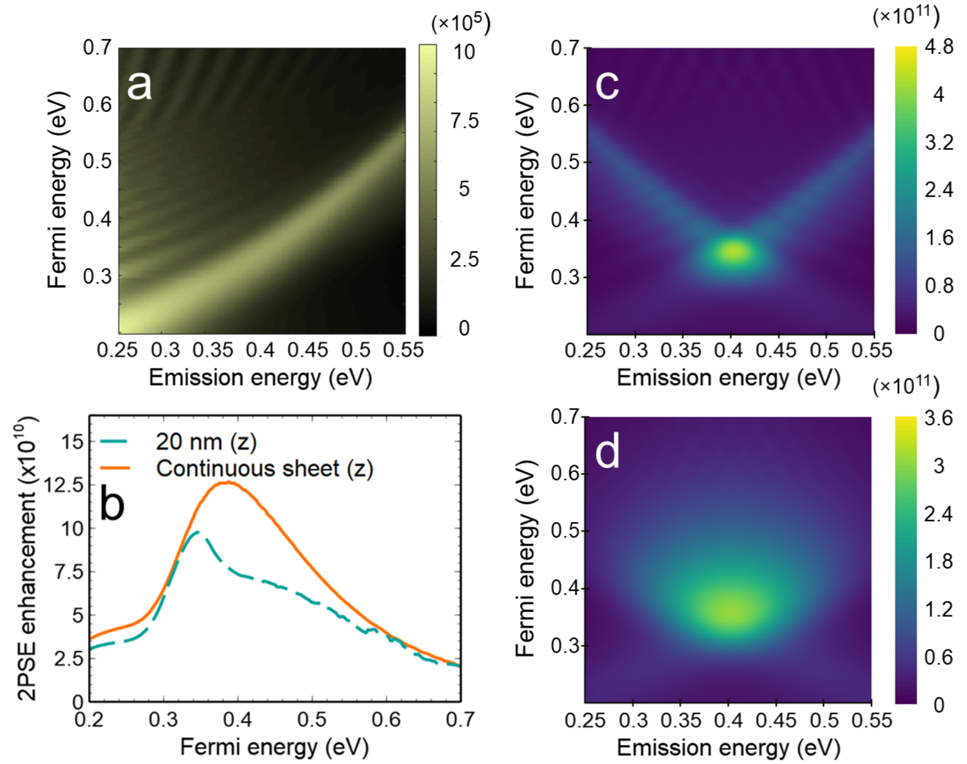


Fig. S4: Results for an emitter in the z-direction (perpendicular to the ribbon or the sheet). (a) Purcell enhancement for the emitter 5 nm beneath 20 nm graphene ribbons. (b) Integrated 2PSE enhancement $\Gamma/\Gamma_0$ for the emitter near 20 nm wide graphene ribbons and near a continuous graphene sheet. (c, d) Differential 2PSE enhancement $\gamma/\gamma_{0,\,max}$ for the emitter near graphene ribbons (c) or a graphene sheet (d). The results in (c) and (d) are normalized by the maximum value of free-space differential 2PSE.

## IV. Variation of Purcell enhancement with graphene nanoribbon width

Fig. S5-S7 demonstrate the effect of change in ribbon width on Purcell enhancement and 2PSE enhancement by replacing the 20 nm ribbons with 14 nm ribbons. The figures show Purcell enhancement, 2PSE enhancement, and differential 2PSE enhancement for all three polarizations of the dipole beneath 14 nm graphene ribbons and compared to a continuous graphene sheet.

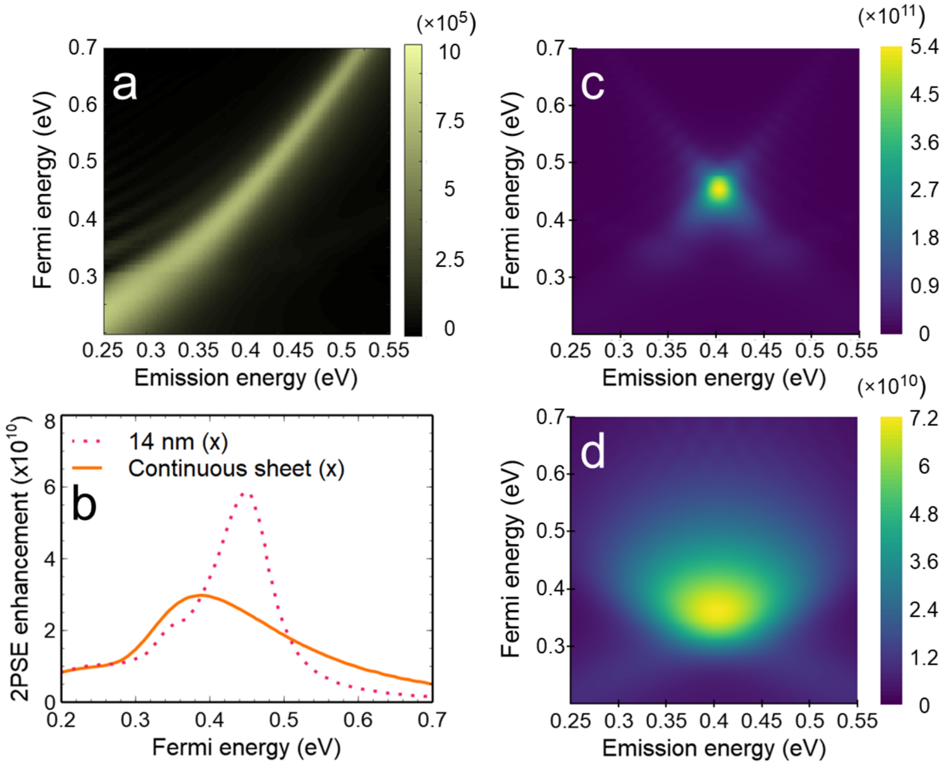


Fig. S5: Results for an emitter in the x-direction (along the ribbon's short axis or parallel to the sheet). (a) Purcell enhancement for the emitter 5 nm beneath 14 nm graphene ribbons. (b) Integrated 2PSE enhancement $\Gamma/\Gamma_0$ for the emitter near 14 nm wide graphene ribbons and near a continuous graphene sheet. (c, d) Differential 2PSE enhancement $\gamma/\gamma_{0,\,max}$ for the emitter near graphene ribbons (c) or a graphene sheet (d). The results in (c) and (d) are normalized by the maximum value of free-space differential 2PSE.

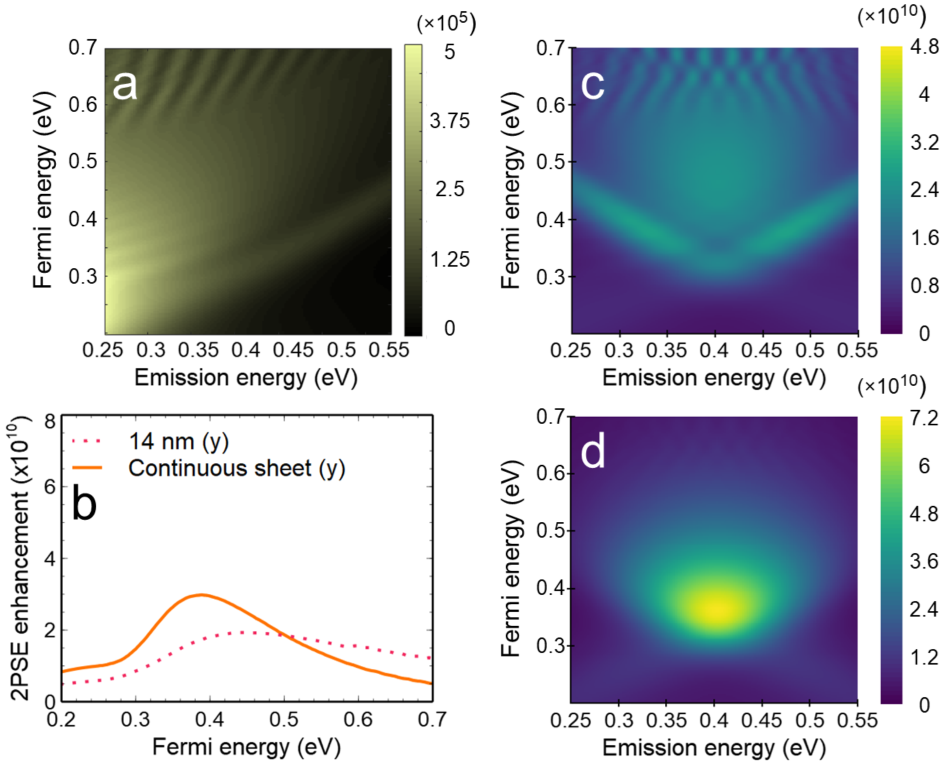


Fig. S6: Results for an emitter in the y-direction (along the ribbon's long axis or parallel to the sheet). (a) Purcell enhancement for the emitter 5 nm beneath 14 nm graphene ribbons. (b) Integrated 2PSE enhancement $\Gamma/\Gamma_0$ for the emitter near 14 nm wide graphene ribbons and near a continuous graphene sheet. (c, d) Differential 2PSE enhancement $\gamma/\gamma_{0,\,max}$ for the emitter near graphene ribbons (c) or a graphene sheet (d). The results in (c) and (d) are normalized by the maximum value of free-space differential 2PSE.

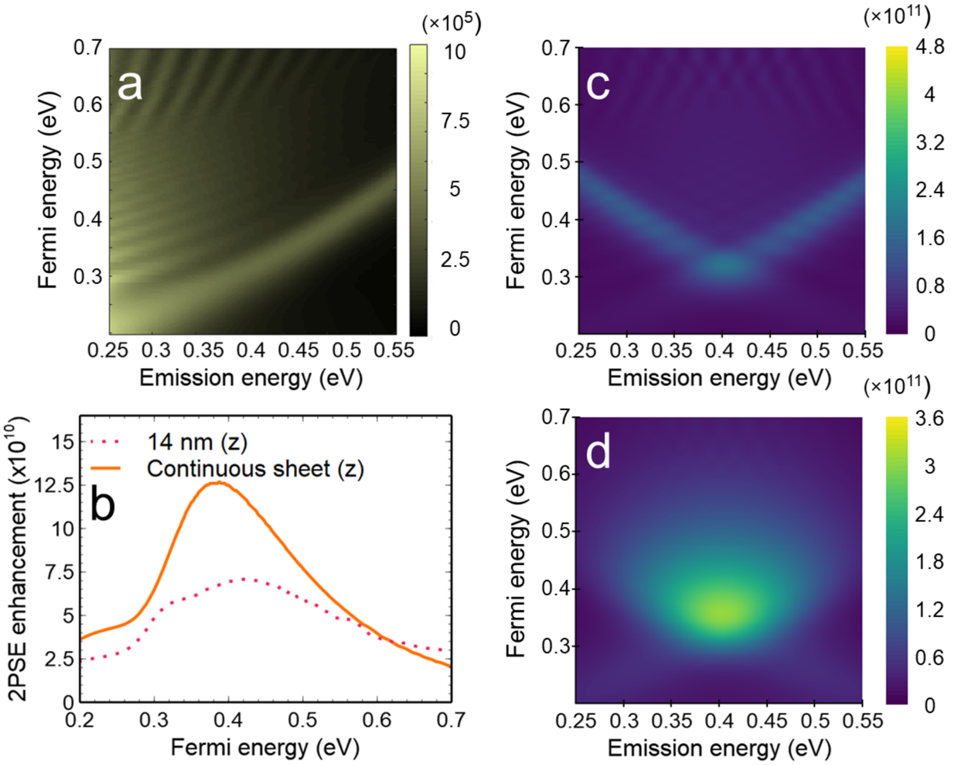


Fig. S7: Results for an emitter in the z-direction (perpendicular to the ribbon or the sheet). (a) Purcell enhancement for the emitter 5 nm beneath 14 nm graphene ribbons. (b) Integrated 2PSE enhancement $\Gamma/\Gamma_0$ for the emitter near 14 nm wide graphene ribbons and near a continuous graphene sheet. (c, d) Differential 2PSE enhancement $\gamma/\gamma_{0,\,max}$ for the emitter near graphene ribbons (c) or a graphene sheet (d). The results in (c) and (d) are normalized by the maximum value of free-space differential 2PSE.

## V. Emission of mixed radiative/nonradiative modes

Fig. 3 of the main paper shows the enhancement of the fully radiative (photon-photon) component of 2PSE in $Er^{3+}$ when modified by graphene ribbons and sheets. Although this mode of radiation provides a potential source of entangled photons, the enhancement generated by this process is relatively weak, with overall enhancement of photon pairs reaching factors of ~ 35 and enhancement of photon pairs near 3.1 μm reaching factors of ~ 400. When we instead consider emission processes in which one decay occurs as a photon and one as a non-radiative plasmon (creating a non-entangled, down-converted photon), we find that the enhancement now reaches factors of ~ $10^6$ for the overall enhancement and ~ $10^7$ for the 3.1 μm enhancement. These results are shown in Fig. S8(a, b) below.

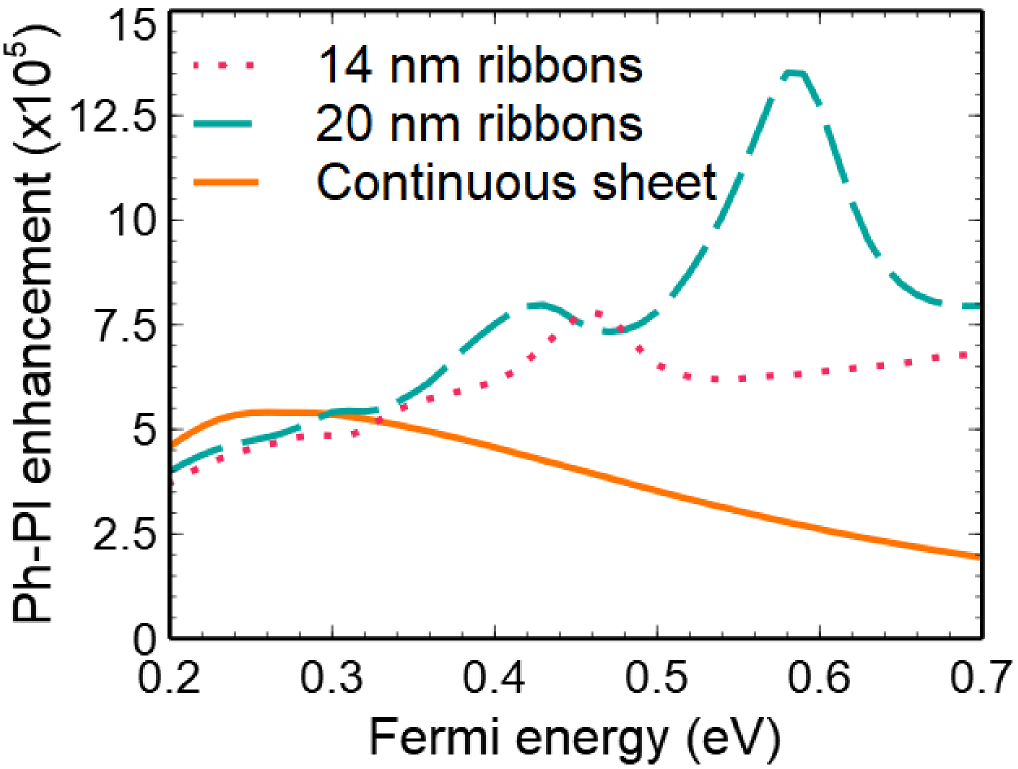


Fig. S8(a): Enhancement of emission in which one photon radiates to free space and the other dissipates as a plasmon. All results consider an $Er^{3+}$ emitter 5 nm away from graphene structures, with all dipole orientations averaged according to Eq. (4).

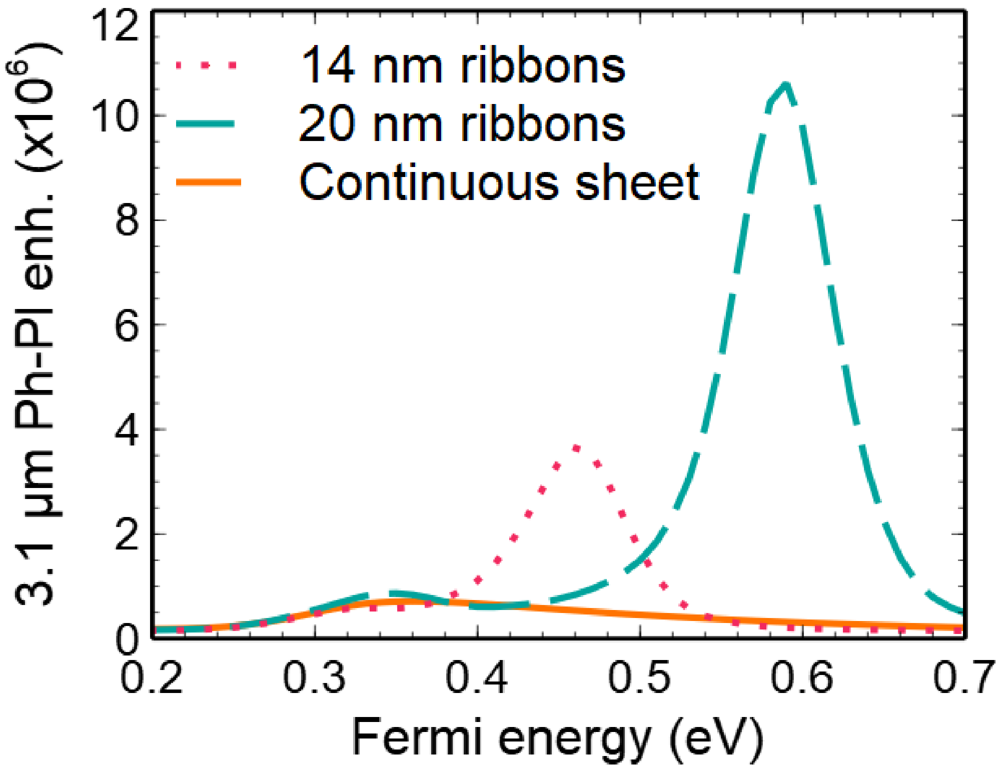


Fig. S8(b): Enhancement of emission in the 3 - 3.2 μm range in which one photon radiates to free space and the other dissipates as a plasmon. All results consider an $Er^{3+}$ emitter 5 nm away from graphene structures, with all dipole orientations averaged according to Eq. (4).

## VI. Variation of total decay rate with graphene nanoribbon width

The overall decay rates for $Er^{3+}$ modified by graphene attributed to both 2PSE and single-transition decay are shown in Fig. 4(c) of the main paper for 20 nm ribbons and a continuous graphene sheet. In Fig. S9, shown below, we present similar results for ribbons with a width of 14 nm. We find behavior that is highly comparable to that of the 20 nm ribbons, as Fig. 4(a) and 4(b) show only weak dependence of overall single-transition decay and 2PSE emission on ribbon width.

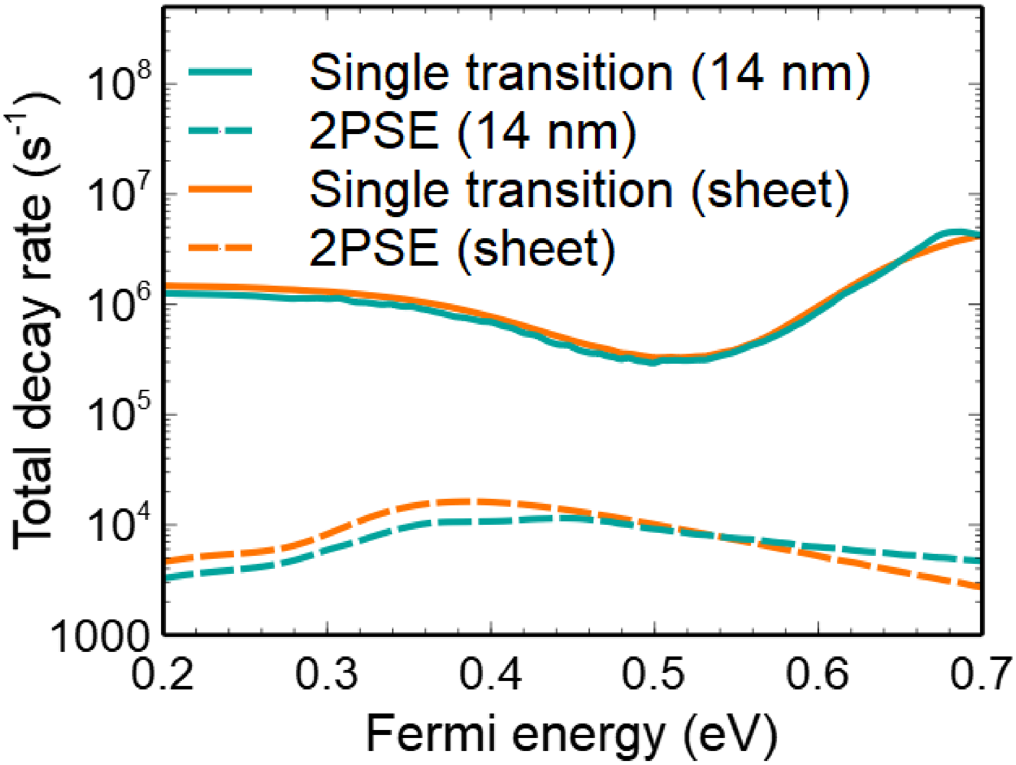


Fig. S9: Total single-transition decay rate compared to total two-photon emission rate in the presence of 14 nm ribbons and a continuous graphene sheet. All results consider an $Er^{3+}$ emitter 5 nm away from graphene structures, with all dipole orientations averaged according to Eq. (4).

## References


[1] R. D. Cowan, *The Theory of Atomic Structure and Spectra* (University of California Press, Berkeley, CA, 1981).

[2] C. Eckart, Reviews of Modern Physics **2**, 305 (1930).

[3] E. Wigner, Zeitschrift für Physik **43**, 624 (1927).
